# Supplementary material for: SQuARM-SGD: Communication-Efficient Momentum SGD for Decentralized Optimization
Source: arXiv:2005.07041 source file (2021-10-11)
Supplement: Supplementary file 1 [file suppl_experiments.tex]

\section{Additional Experiments} \label{suppl_experiments}
In this section, we provide experimental results for comparison of our algorithm SQuARM-SGD to CHOCO-SGD \cite{koloskova_decentralized_2019} and vanilla-SGD for CIFAR-10 dataset \cite{cifar} (along with wall-clock time comparison), and for MNIST dataset to optimize a convex objective. In Subsection \ref{suppl_cifar_acc}, we describe the setup for training on CIFAR-10 dataset, and compare schemes based on their training performance and test-accuracy vs. communication trade-off. Subsection \ref{suppl_cifar_time} provides comparison for wall-clock time when training on CIFAR-10 dataset with a rate-limited communication pipeline between the worker nodes. This is typically the case in edge computing applications where efficient decentralized learning is desired, as significant communication rate (bandwidth) constraints may exist which cause the communication time itself to be a bottleneck.   
Lastly, Subsection \ref{suppl_mnist_acc} provides comparison plots for performance on MNIST dataset for a convex objective.

% {\bf Wall-clock time comparison}
%An important application for efficient decentralized learning arises in edge computing applications which may have significant communication rate (bandwidth) constraints. Typical hardware processors used in large scale learning tasks have a clock speed in GHz, while the allowable communication rate in such settings may be much lower. For example, the average cellular LTE rate is within 1-5 Mbps, which is orders below in magnitude from the computation rate, thus posing the communication time itself as the major bottleneck. Thus, such settings call for need of schemes which are highly communication efficient to save on communication time over bandlimited channels. 

\subsection{Experiments on CIFAR-10 dataset} \label{suppl_cifar_acc}

{\bf Setup.}
We match the setting in CHOCO-SGD \cite{koloskova_decentralized_2019} and perform our experiments on the CIFAR-10 \cite{cifar} dataset and train a ResNet20 \cite{wen2016learning} model with $n=8$ nodes connected in a ring topology. The training is done on TitanRTX GPUs. Learning rate is initialized to $0.1$, following a schedule consisting of a warmup period of 5 epochs followed by piecewise decay of 5 at epoch 200 and 300 and we stop training at epoch 400. The SGD algorithm is implemented with momentum with a factor of 0.9 and mini-batch size of 256. 
SQuARM-SGD consists of $H=5$ local iterations followed by checking for a triggering condition, and then communicating with the composed $SignTopK$ operator, where we take top 1\% elements of each tensor and only transmit the sign and norm of the result. The triggering threshold follows a schedule piecewise constant: initialized to 2.5 and increases by 1.5 after every 20 epochs till 350 epochs are complete; while maintaining that $c_t < \nicefrac{1}{\eta}$ for all $t$. We compare performance of SQuARM-SGD against CHOCO-SGD with $Sign$, $TopK$ compression (taking top 1\% of elements of the tensor) and decentralized vanilla SGD \cite{lian2017can}. 
We also provide a plot for using the composed $SignTopK$ operator without event-triggering titled `SQuARM-SGD (Sign-TopK)' for comparison.

\begin{figure}[H]
	\subfigure[] { \label{fig:lo-noncvx} \includegraphics[scale=0.45]{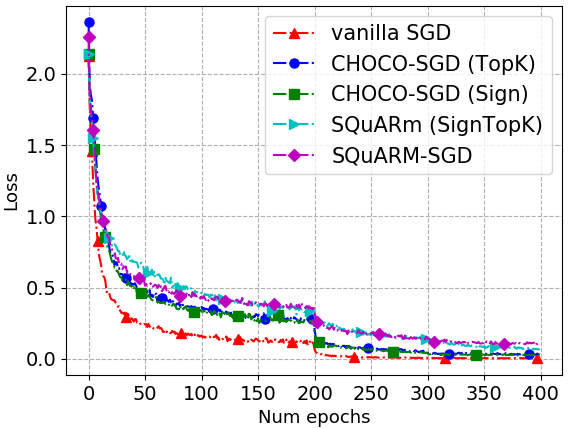}} \hfill
	\subfigure[] { \label{fig:te-logbits-noncvx} \includegraphics[scale=0.45]{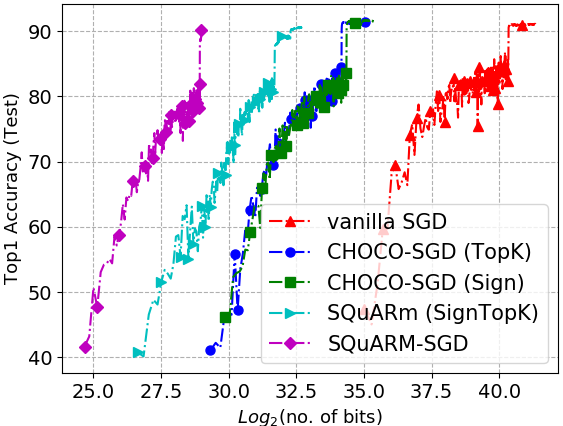}} \hfill
%	\subfigure[] { \label{fig:lo-time-noncvx} \includegraphics[scale=0.45]{suppl_noncvx_loss_time-plots.png}} \hfill
%	\subfigure[] { \label{fig:te-time-noncvx} \includegraphics[scale=0.45]{suppl_noncvx_tacc_time-plots.png}}
	\caption{These plots are for training a ResNet20 model (non-convex objective) on the CIFAR-10 dataset. Figure~\ref{fig:lo-noncvx} and \ref{fig:te-logbits-noncvx} show training loss vs.\ epochs and Top-1 accuracy vs.\ total number of bits communicated, respectively. 
%		In Figure~\ref{fig:lo-time-noncvx} and Figure~\ref{fig:te-time-noncvx}, we compare training loss vs time (in sec) and Top-1 accuracy vs time (in sec) respectively for the different schemes. 
	}
	\label{fig:figures_suppl_noncvx}
\end{figure}

{\bf Results.}
We plot the global loss function evaluated at the average parameter vector across nodes in Figure \ref{fig:lo-noncvx}, where we observe SQuARM-SGD converging at a similar rate as CHOCO-SGD and vanilla decentralized SGD. Figure \ref{fig:te-logbits-noncvx} shows the performance for a given bit-budget, where we show the Top-1 test accuracy%
 \footnote{Here, Top-1 accuracy corresponds to the percentage of test examples for which the correct label is equal to the label considered most probable by the model.} as a function of the total number of bits communicated. For Top-1 test-accuracy of around 90\%, SQuARM requires about 40$\times$ less bits than CHOCO with $Sign$ or $TopK$ compression, and around 3K$\times$ less bits than vanilla decentralized SGD to achieve the same Top-1 accuracy. \\

 \subsection{Wall-clock time comparison for CIFAR-10 dataset with rate-limited communication} \label{suppl_cifar_time}
 
 \begin{figure}[H]
%	\subfigure[] { \label{fig:te-logbits-noncvx2}
% 	\includegraphics[scale=0.37]{suppl_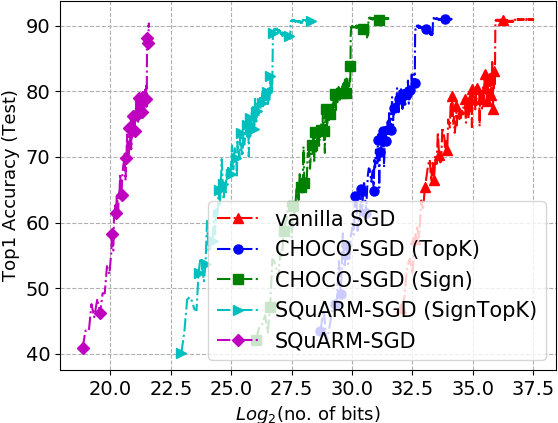}} \hfill
 \subfigure[] { \label{fig:te-logbits-logcommtime}
	\includegraphics[scale=0.45]{suppl_noncvx_tacc-logcommtime.png}} \hfill
 	\subfigure[] { \label{fig:te-time-noncvx} \includegraphics[scale=0.45]{suppl_noncvx_tacc_time-plots.png}}
 	\caption{
% 		These plots are for training a ResNet20 model (non-convex objective) on the CIFAR-10 dataset. 
 	Figure~\ref{fig:te-logbits-logcommtime} shows Top-1 accuracy as a function of total communication time through a bandlimited rate pipe of 100Kbps.
 	 Figure~\ref{fig:te-time-noncvx} shows the total time (computation + communication) required to reach a target Top-1 accuracy of $90$\% for the different schemes. 
 }
 	\label{fig:figures_suppl_noncvx2}
 \end{figure}

  {\bf Setup.} We follow the same setup as stated in the Subsection \ref{suppl_cifar_acc}, and further we assume that the communication between workers is rate-limited to 100Kbps. This is typical {\em average} rate of wireless edge devices sharing a common bandwidth with other devices, therefore devices cannot have sustained high rates.
 
 {\bf Results.}
 Figure~\ref{fig:te-logbits-logcommtime} shows the Top-1 accuracy as a function of time required to communicate bits through a rate pipe constrained to 100Kbps. We observe that, to reach a target accuracy of $90$\%, SQuARM-SGD saves a factor of around $40 \times$ in communication time compared to CHOCO-SGD with $Sign$ or $TopK$ sparsifier, and around  $3$K$\times$ less communication time than vanilla SGD. Thus, there is a significant saving in communication time for SQuARM-SGD compared to other schemes when communicating over typical rate limited channels.
This result is almost a direct translation of the savings in the number of bits needed for training.

In Figure~\ref{fig:te-time-noncvx}, we plot Top-1 accuracy vs.\ the wall-clock time, when the communication between workers is over the rate-limited pipelines (limited to 100Kbps). The wall-clock time includes the total time taken in both computation and communication; note that this includes time required to setup the communication (\emph{e.g.,} interrupts in processing) and other overheads, and not just the airtime (time to transmit the bits) for the communication as done in Figure~\ref{fig:te-logbits-logcommtime}. We observe that, to reach a target test-accuracy of around $90$\%, SQuARM-SGD saves a factor of around $30 \times$ in total time compared to CHOCO-SGD with $Sign$ or $TopK$ compression, and around 2.5K$\times$ compared to vanilla-SGD. 
The significant advantage to our method comes due to efficient transmission over the rate constrained pipeline.

Note that one can expect uncompressed schemes to do better in terms of computation time, but as shown in the plots above, the high communication time required in uncompressed schemes on rate-constrained links would far outweigh the advantage due to computation time. As a result, the total time required by SQuARM-SGD (that incorporates compression and infrequent communication) to reach a certain accuracy would be significantly smaller than either the uncompressed schemes or the ones using infrequent communication or both.

\subsection{Experiments for convex objective on MNIST dataset} \label{suppl_mnist_acc}
\begin{figure}[ht]
	\centering
	\subfigure[] { \label{fig:lo-cvx} \includegraphics[scale=0.45]{suppl_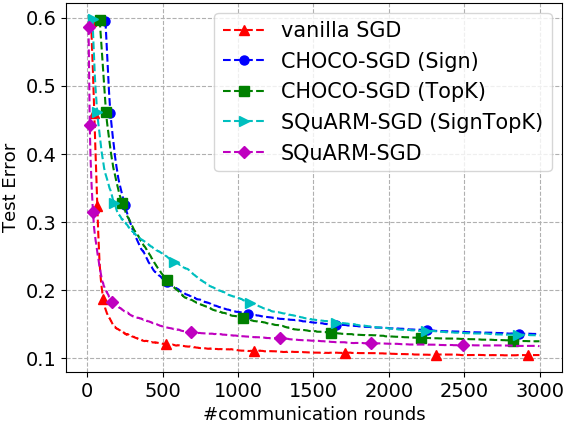}} \hfill
	\subfigure[] { \label{fig:te-logbits-cvx} \includegraphics[scale=0.45]{suppl_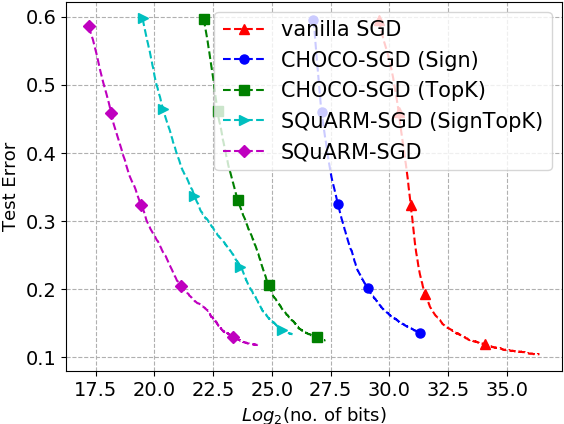}}
	\caption{Figure \ref{fig:lo-cvx} and \ref{fig:te-logbits-cvx} are for convex objective simulated on the MNIST dataset, where we plot test error vs number of communication rounds and test error vs total number of bits communicated, respectively, for different algorithms.}
	\label{fig:figures_suppl_cvx}
\end{figure}
{\bf Setup.}
We run SQuARM-SGD on MNIST dataset and use multi-class cross-entropy loss to model the local objectives $f_i, i\in[n]$. We consider $n=60$ nodes connected in a ring topology, each processing a mini-batch size of 5 per iteration and having heterogeneous distribution of data across classes. We work with $\eta_t = 1/(t+100)$ (based on grid search) and synchronization index $H=5$. For SQuARM-SGD, we use the composed operator $SignTopK$ (\cite{basu_qsparse-local-sgd:_2019}) with $k=10$ (out of 7840 length vector for MNIST dataset)
For our experiments, we set the triggering constant $c_0 = 5000$ in SQuARM-SGD (line 7) and keep it unchanged until a certain number of iterations and then increase it periodically;
while still maintaining that $c_t \eta_t^2$ decreases with $t$ (as $c_t$ is  $o(t)$ ) .

{\bf Results.}
In Figure \ref{fig:lo-cvx}, we observe SQuARM-SGD can reach a target test error in fewer communication rounds while converging at a rate similar to that of vanilla SGD. The advantage to SQuARM-SGD comes from the significant savings in the number of bits communicated to achieve a desired test error, as seen in Figure \ref{fig:te-logbits-cvx}: to achieve a test error of around 0.12, SQuARM-SGD gets 120$\times$ savings as compared to CHOCO-SGD with $Sign$ quantizer, around 10-15$\times$ savings than CHOCO-SGD with $TopK$ sparsifier, and around 1000$\times$ savings than vanilla decentralized SGD.
