# Supplementary material for: SQuARM-SGD: Communication-Efficient Momentum SGD for Decentralized Optimization
Source: arXiv:2005.07041 source file (2021-10-11)
Supplement: Supplementary file 2 [file appendix_expts.tex]

\section{Additional experiments} \label{supp_add_expts}

\subsection{Effect of local iterations $(H)$ on SQuARM-SGD}

\begin{figure}[t]
	\centering
	\includegraphics [width=0.4\linewidth]{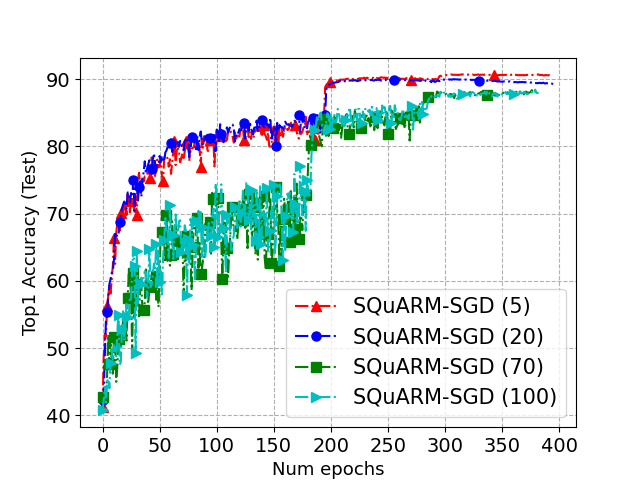}
	\caption{Comparison of Test accuracies for different values of $H$ for SQuARM-SGD.}
	\label{rev2:fig1}
\end{figure}

We consider the same setting as in our main paper, and compare the performance of SQuARM-SGD for $H \in \{5,20,70,100\}$. We observe that the proposed scheme works well for reasonable values of $H$, which taking large $H$ can slightly hurt the performance due to very infrequent information exchange among clients.

}
